# Supplementary material for: Dual-Solver: A Generalized ODE Solver for Diffusion Models with Dual Prediction
Source: arXiv:2603.03973 source file (2026-03-04)
Supplement: Supplementary file 1 [file gmdit_figs.tex]

% 헤더: 좌(모델명) ↔ 우(Acc/FID), Acc는 셋째자리까지 표기
\newcommand{\RowImageWithHeader}[6]{%
  \begin{subfigure}[t]{\textwidth}
    \noindent
    {\footnotesize \texttt{#3}\hfill Top-5 Acc.: #4\%\ \ \ FID: #5}\\[-2pt]
    \includegraphics[width=\textwidth]{#2}
  \end{subfigure}\vspace{3pt}%
}

% ========= Page 1 =========
\begin{figure*}[p]
\centering

% FID@3 ascending (앞 10개)
\RowImageWithHeader{r14}{appendix/accuracy/gmdit_figs/which13.png}{RegNet\_Y\_800MF\_Weights.IMAGENET1K\_V1}{93.136}{9.40}{}
\RowImageWithHeader{r15}{appendix/accuracy/gmdit_figs/which14.png}{MobileNet\_V3\_Large\_Weights.IMAGENET1K\_V2}{92.566}{9.44}{}
\RowImageWithHeader{r12}{appendix/accuracy/gmdit_figs/which11.png}{ResNet152\_Weights.IMAGENET1K\_V1}{94.046}{9.49}{}
\RowImageWithHeader{r11}{appendix/accuracy/gmdit_figs/which10.png}{RegNet\_Y\_3\_2GF\_Weights.IMAGENET1K\_V1}{94.576}{9.50}{}
\RowImageWithHeader{r16}{appendix/accuracy/gmdit_figs/which15.png}{RegNet\_Y\_400MF\_Weights.IMAGENET1K\_V1}{91.716}{9.50}{}
\RowImageWithHeader{r18}{appendix/accuracy/gmdit_figs/which17.png}{MobileNet\_V2\_Weights.IMAGENET1K\_V1}{90.286}{9.52}{}
\RowImageWithHeader{r10}{appendix/accuracy/gmdit_figs/which9.png}{RegNet\_Y\_8GF\_Weights.IMAGENET1K\_V1}{95.048}{9.54}{}
\RowImageWithHeader{r09}{appendix/accuracy/gmdit_figs/which8.png}{RegNet\_Y\_32GF\_Weights.IMAGENET1K\_V1}{95.340}{9.55}{}
\RowImageWithHeader{r13}{appendix/accuracy/gmdit_figs/which12.png}{ResNet101\_Weights.IMAGENET1K\_V1}{93.546}{9.59}{}
\RowImageWithHeader{r17}{appendix/accuracy/gmdit_figs/which16.png}{RegNet\_X\_400MF\_Weights.IMAGENET1K\_V1}{90.950}{9.60}{}

\caption{\textbf{Sampling results by classifier.} Classifier weights, top-5 accuracy, and FID are reported; entries are sorted by ascending FID.}
\label{fig:by_classifier1}

\end{figure*}

% ========= Page 2 (continued) =========
\begin{figure*}[p]
\ContinuedFloat
\centering

% FID@3 ascending (뒤 10개)
\RowImageWithHeader{r06}{appendix/accuracy/gmdit_figs/which5.png}{RegNet\_Y\_16GF\_Weights.IMAGENET1K\_V2}{96.328}{9.63}{}
\RowImageWithHeader{r08}{appendix/accuracy/gmdit_figs/which7.png}{Swin\_T\_Weights.IMAGENET1K\_V1}{95.776}{9.65}{}
\RowImageWithHeader{r07}{appendix/accuracy/gmdit_figs/which6.png}{Swin\~V2\_T\_Weights.IMAGENET1K\_V1}{96.132}{9.73}{}
\RowImageWithHeader{r03}{appendix/accuracy/gmdit_figs/which2.png}{RegNet\_Y\_16GF\_Weights.IMAGENET1K\_SWAG\_LINEAR\_V1}{97.244}{9.97}{}
\RowImageWithHeader{r04}{appendix/accuracy/gmdit_figs/which3.png}{ConvNeXt\_Base\_Weights.IMAGENET1K\_V1}{96.870}{10.28}{}
\RowImageWithHeader{r01}{appendix/accuracy/gmdit_figs/which0.png}{ViT\_H\_14\_Weights.IMAGENET1K\_SWAG\_E2E\_V1}{98.694}{10.71}{}
\RowImageWithHeader{r20}{appendix/accuracy/gmdit_figs/which19.png}{AlexNet\_Weights.IMAGENET1K\_V1}{79.066}{11.20}{}
\RowImageWithHeader{r05}{appendix/accuracy/gmdit_figs/which4.png}{EfficientNet\_B5\_Weights.IMAGENET1K\_V1}{96.628}{11.53}{}
\RowImageWithHeader{r19}{appendix/accuracy/gmdit_figs/which18.png}{ShuffleNet\_V2\_X1\_0\_Weights.IMAGENET1K\_V1}{88.316}{11.57}{}
\RowImageWithHeader{r02}{appendix/accuracy/gmdit_figs/which1.png}{RegNet\_Y\_128GF\_Weights.IMAGENET1K\_SWAG\_LINEAR\_V1}{97.844}{12.99}{}
\caption{\textbf{Sampling results by classifier.} (continued).}
\label{fig:by_classifier2}
\end{figure*}
